# Supplementary material for: Embedding Lexical Features via Low-Rank Tensors
Source: arXiv:1604.00461 source file (2016-04-02)
Supplement: Supplementary file 1 [file appendix.tex]

\section*{Appendix A: Gradients for the Training of Low-rank Tensors}

\begin{table}[tbp]
  \small
  \centering
  %\begin{tabular}{|l|p{1.7cm}|p{2.9cm}|p{5.8cm}|}
  \begin{tabular}{|c|c|}
  \hline
    \bf Symbol & {\bf Description}\\
     \hline
    $\cT$  &Parameter tensor\\
    $\bW{i}$ & Transformation on the $i$th view\\    
    $\bh_i$ & Hidden representation on the $i$th view\\
    $d_i$ & Dimension of inputs on the $i$th view\\ 
    $r_i$ & Dimension of $\bh_i$ (Tucker)\\
    $r$ & Dimension of $\bh_i$s (CP)\\ 
    $g$ & Core tensor (Tucker)\\
    $\phi$ & Lexical feature\\
    $e_{\phi}$ & feature representation (one-hot or LRFR) of $\phi$\\
    $D$ & Training data set\\
    $(\bx, y)$& A training instance\\
    $\times_i$ & the tensor $i$-mode product\\
    $\circ$ & Element-wise multiplication\\
    $\odot$ & Dot Product \\
    \hline
  \end{tabular}
  \caption{Reference for mathematical notations.}
  \label{tab:notations}
  \vspace{-0.25in}
\end{table}

\paragraph{An Equivalent Form of Scoring Function}
For computational efficiency, we re-write the scoring function as follows. Let
$\mathbf{\Phi}^{(1)}(i) = \{\phi \in F_1|w({\phi}) = \v_i\} $
denote the set of all unigram lexical features the lexical parts of which are the word $\v_i$ in $\bx$. 
Similarly we have $\mathbf{\Phi}^{(2)}(i, j) = \{\phi \in F_2|w_1(\phi) = \v_i\ \textrm{and}\ w_2(\phi) = \v_j\}$
for all bigram lexical features where the first lexical parts are word $\v_i$ and the second lexical
parts are word $\v_j$.
We denote $\mathbf{u}^{(1)}(i)$ and $\mathbf{u}^{(2)}(i,j)$ as the corresponding vector of non-lexical
parts in $\mathbf{\Phi}^{(1)}(i)$ and $\mathbf{\Phi}^{(2)}(i, j)$ respectively.

In the rest of this section we take feature sets with only unigram and bigram lexical features as an example,
while the idea can be applied to other $n$-gram lexical features as well.
Assume we have $M$ words in $\bx$, the prediction function can be written as

\vspace{-0.2in}
\begin{small}
\begin{align}
%&s(\bx,y;\cT) = \sum_{i=1}^n \sum_{\phi \in F_i(\bx,y)} s(\phi;\cT_i) \nonumber\\
&P(\y|\bx;\cT_1,\cT_2)  \nonumber\\
\! \propto&\! \exp\left \{ \sum_{\phi \in F_1(\bx,\y)} s(\phi; \cT_1) + \sum_{\phi \in F_2(\bx,y)} s(\phi; \cT_2) \right \} \nonumber \\
\! \propto&\! \exp\left \{ \sum_{i=1}^{M_1} \cT_1 \times_{\l} \y \times_f \mathbf{u}^{(1)}(i) \times_{\w} \be_{\v_i} \right. \label{eq:train-equivalent}\\
& +\left. \sum_{i=1}^{M}\sum_{j=1}^M \cT_2 \times_{\l} \y \times_f \mathbf{u}^{(2)}(i,j) \times_{\w_1} \be_{\v_i} \times_{\w_2} \be_{\v_j}\right \} \nonumber
%P(y|\bx;\cT) &\! \propto\! \exp\left \{ \sum_{i=1 }^T g \times_y \bh_y \times_f \bh_{\mathbf{f}^{(i)}} \times_w \bh_{w_i} \right \} \nonumber \\
%& \! \propto\! \exp\left \{ (g \times_y \bh_y)  \odot \left( \sum_{i=1}^T \bh_{\mathbf{f}^{(i)}} \otimes \bh_{w_i} \right) \right \}. 
\end{align}
\end{small}
\vspace{-0.1in}
%
% =======
%For computational efficiency, we can re-write the equation as follows:
%Denote $\mathbf{f}_{w_i} = \sum_{\{lf|w_{lf} = w_i\}} f_{lf}$, which is the unlexical parts associated with each word. Assume we have $T$ different words, we can re-write the equation as:
%\begin{align}
%&P(y|\bx;\cT) \propto \exp\left \{ \sum_{i=1 }^T g \times_y \bh_y \times_f \bh_{\mathbf{f}_{w_i}} \times_e \bh_{e_{w_i}} \right \} \nonumber \\
%&  = \exp\left \{ (g \times_y \bh_y)  \odot \left( \sum_{i=1}^T \bh_{\mathbf{f}_{w_i}} \otimes \bh_{e_{w_i}} \right) \right \}
%\label{eq:train-equivalent}
%>>>>>>> 8f2118e5e4ec37a5d875acbb75934e9e42937244

\paragraph{Stochastic Gradient for Low-rank Tensors}
We optimize the following log-likelihood objective:
\begin{align}
\textstyle \mathcal{L}({\cT_1,\cT_2 }) = - \frac{1}{|D|} \sum_{(\y, \bx )\in D} \log P(\y | \bx; {\cT_1,\cT_2}), \nonumber
\vspace{-0.1 in}
\end{align}
where $D$ is the training set. For
each instance $(\y, \bx)$ we compute the gradient of the log-likelihood $\ell = -\log P(\y | \bx;
{\cT_1,\cT_2})$. 

We define the vector 
%$\mathbf s=\left[ \bW_ \bh_y\sum_i T_y \odot (\mathbf{g_i} \otimes e_{w_i}) \right]_{1\le y \le L}$, 
$\bs$, where $\bs_{\y'} = \bs(\bx,\y';\cT_1,\cT_2)= \sum_{\phi \in F_1(\bx,\y')} s(\phi; \cT_1) + \sum_{\phi \in F_2(\bx,\y')} s(\phi; \cT_2)$,
%= \left[ \sum_{i=1}^T g \times_y \bh_{y'} \times_f \bh_{\mathbf{f}^{(i)}} \times_w \bh_{w_i} \right]$, 
which yields ${\partial \ell}/{\partial \mathbf s} =\left[ (
    I[\y=\y']-P(\y' | \bx; \cT_1,\cT_2) )
\right]_{ \y' \in L}^T, \nonumber$
where the indicator function $I[z]$ equals to 1 if $z$
is true and zero otherwise. 
Taking the view of non-lexical features as example, 
we have the following stochastic gradients, where \lrfcmt\ is mainly for unigram features and
\lrfcmcp\ works for any $n$-gram features (here we take bigram features as an example):
\paragraph{\lrfcmt}
For a component tensor $\cT = g \times \bW{y} \times_f \bW{f} \times_w \bW{e}$ for unigram features, we have
%\begin{small}
\begin{align}
\frac{\partial \ell}{\partial g} &= \left( \sum_{\y'=1}^L \frac{\partial \ell}{\partial \bs_{\y'}} \bh_{\y'}^{(l)} \right) 
\otimes \left(\sum_{i=1}^M \bh_{\mathbf{u}^{(1)}(i)}^{(f)} \otimes \bh_{\v_i}^{(1)} \right), \nonumber
%\frac{\partial \ell}{\partial g_2} &= \left( \sum_{y'=1}^L \frac{\partial \ell}{\partial \bs_{y'}} \bh_{2y'} \right) 
%\otimes \left(\sum_{i=1}^M\sum_{j=1}^M \bh_{2\mathbf{f}^{(2)}(i,j)} \otimes \bh_{2w_i} \right), \nonumber
\end{align}
\begin{align}
\frac{\partial \ell}{\partial \bW{f}[:,u]} &= \sum_{i=1}^M \frac{\partial \ell}{\partial \bh_{\mathbf{u}^{(1)}(i)}^{(f)}} \frac{\partial \bh_{\mathbf{u}^{(1)}(i)}^{(f)}}{\partial \bW{f}[:,u]} \nonumber\\
&= \sum_{i=1}^M\sum_{\y'} \left( I[u \in \mathbf{u}^{(1)}(i)] \frac{\partial \ell}{\partial \mathbf{s}_{\y'}} \right. \nonumber\\
&\quad\quad \left. \cdot g \times_l \bh_{\y'}^{(l)} \times_{w} \bh_{\v_i}^{(1)} \right). 
\end{align}
%\end{small}
where $\bh_{\y}^{(l)} = \bW{\y} \y$, $\bh_{\v_i}^{(1)} = \bW{e} \v_i$, and $\bh_{\mathbf{u}^{(1)}(i)}^{(f)} = \bW{f} \mathbf{u}^{(1)}(i)$. Similar definitions work for the other $\bh$s. The gradients for the $\bW{}$s on the other two views have similar forms as ${\partial \ell}/{\partial \bW{f}}$.
%and

\paragraph{\lrfcmcp}
For a component tensor $\cT_n = \bW{\l}^{(n)} \otimes \bW{f}^{(n)} \otimes \bW{e_1}^{(n)} \ldots \otimes \bW{e_n}^{(n)}$, taking bigram features as an example ($n$=2), we have the following gradients for $\cT_2$:
\begin{small}
\begin{align}
\frac{\partial \ell}{\partial \bW{f}^{(2)}[:,u]} %&= \sum_{i=1}^n \frac{\partial \ell}{\partial \bh_f} \frac{\partial \bh_f}{\partial \bW{f}} \nonumber\\
&= \sum_{i=1}^M \sum_{j=1}^M \sum_{\y'} I[u \in \mathbf{u}^{(2)}] \frac{\partial \ell}{\partial \mathbf{s}_{\y'}} \left( \bh_{\y'}^{(l)} \odot \bh_{\v_i}^{(1)}  \odot \bh_{\v_j}^{(2)} \right). \nonumber
\end{align}
\end{small}
Similarly we can get the gradients for the $\bW{}^{(n)}$s on the other views. 

\section*{Appendix B: Derivation of Equation \ref{eq:fcm_ngram} and \ref{eq:fcmcp_ngram}}
\paragraph{\lrfcmt}
The derivation of scoring a lexical feature with low-rank tensor with Tucker-form is straightforward as below:
\begin{align}
&\hspace*{-14pt}\textstyle \!s(\y, \x, \w_1,\cdots, \w_n; g,{\bW{\l}},{\bW{f}}, {\{\bW{i}\}_{i=1}^n})  \nonumber\\ 
=&\ \cT \times_{\l} \y \times_f \x \times_{\w_1} \w_{1} \times_{\w_2} \cdots \times_{\w_n} \w_n \nonumber \\
=&\ \left(g \times_{\l} \bW{\l} \times_f \bW{f}  \times_{\w_1} \cdots \times_{\w_n} \bW{n} \right) \nonumber \\
&\quad \times_{\l} \y \times_f \x \times_{\w_1} \w_{1} \times_{\w_2} \cdots \times_{\w_n} \w_n \nonumber \\
=&\ g \times_{\l} (\bW{\l} \y) \times_f (\bW{f} \x) \times_{\w_1} (\bW{e_1} \w_1) \times_{\w_2} \cdots \nonumber \\
&\quad  \times_{\w_n} (\bW{n} \w_n) \nonumber \\
%&\quad \times_\ell \y \times_f \x \times_{\w_1} \w_{1} \ldots \times_{\w_n} \w_n \nonumber \\
=&\ g \times_{\l} \bh^{(\l)}_\y \times_f \mathbf{h}^{(f)}_\x  \times_{\w_1} \bh^{(1)}_{\w_1} \cdots\times_{\w_n} \bh^{(n)}_{\w_n},
%  \label{eq:fcm_ngram}
\end{align}

\paragraph{\lrfcmcp}
Here we show the derivation of scoring a lexical feature with low-rank tensor with CP-form:
%\vspace{-0.2in}
\begin{small}
\begin{align}
&\textstyle \!s({\w}_{1,\cdots,n}, \x, \y;\! {\{\bW{e_i}\}},{\bW{f}},{\bW{l}})  \nonumber\\ 
=& \hat{\cT} \times_l \y \times_f \x \times_{\w_1} \w_{1} \ldots \times_{\w_n} \w_n \nonumber \\
=& \left(\sum_{j=1}^r \bW{l}[j,:] \otimes \bW{f}[j,:]  \otimes \bW{e_1}[j,:] \ldots \otimes \bW{e_n}[j,:] \right) \nonumber \\
&\quad \times_l \y \times_f \x \times_{w_1} \w_{1} \ldots \times_{w_n} \w_n \nonumber \\
=& \sum_{j=1}^r \left( \bW{l}[j,:]\cdot \y \times \bW{f}[j,:]\cdot \x \right. \nonumber \\
&\left.  \times \bW{e_1}[j,:] \cdot \w_1 \ldots \times \bW{e_n}[j,:]\cdot \w_n  \right) \nonumber \\
%=& \sum_{j=1}^r \left( \bW{l}[j,:]\cdot y \times \bW{f}[j,:]\cdot f \right. \nonumber \\
%&\left.  \times \bW{e_1}[j,:] \cdot w_1 \ldots \times \bW{e_n}[j,:]\cdot w_n  \right) \nonumber \\
%&\quad \times_l y \times_f f \times_{w_1} w_{1} \ldots \times_{w_n} w_n \nonumber \\
=& \sum_{j=1}^r \left( \bh_{\y}^{(l)}[j] \times \mathbf{h}_{\x}^{(f)}[j] \times\bh_{\w_1}^{(1)}[j] \ldots \times \bh_{\w_n}^{(n)}[j] \right) \nonumber \\
=& \sum_{j=1}^r \left( \bh_{\y}^{(l)} \circ \mathbf{h}_{\x}^{(f)} \circ \bh_{\w_1}^{(1)} \ldots \circ \bh_{\w_n}^{(n)} \right)_j. \nonumber
\end{align}
\end{small}
\vspace{-0.1in}

Here $\bW{l}[j,:]\cdot \y$ is the inner product between vectors. We take the view of $\y$ as example to show why above equation holds.
The second equation is because that for $\cT_j = \bW{l}[j,:] \otimes \bW{f}[j,:]  \otimes \bW{e_1}[j,:] \ldots \otimes \bW{e_n}[j,:]$, we will have 
\begin{align}
&(\cT_j \times_l \y)_{i_2\ldots i_{n+2}} \nonumber\\
=& (\cT_j)_{i_1i_2\ldots i_{n+2}} I[\y = i_1]= (\cT_j)_{\y i_2\ldots i_{n+2}},\nonumber
\end{align}
while
\begin{align}
(\cT_j)_{\y i_2\ldots i_{n+2}} = \left(\bW{l}[j,:]\cdot \y\right) \left(\bW{f}[j,:]  \right. \nonumber\\
\left. \otimes\bW{e_1}[j,:] \ldots \otimes \bW{e_n}[j,:]\right)_{i_2\ldots i_{n+2}}. \nonumber
\end{align}
Therefore $(\cT_j)_{\y i_2\ldots i_{n+2}}$ can be viewed as a element from an $(n+1)$-way tensor $\cT_j(\y) = (\bW{l}[j,:]\cdot \y) \left(\bW{f}[j,:] \otimes\bW{e_1}[j,:] \ldots \otimes \bW{e_n}[j,:]\right)$.
Then we can recursively apply above derivation to each view and get the product among $n+2$ numbers.
The forth equation is from $\bW{l}[j,:]\cdot \y =  \bW{l}[j,\y]$ and $\bh_{\y}^{(l)} = \bW{l}[:,\y]$, therefore the $j$th element of $\bh_{\y}^{(l)}$ is $\bh_{\y}^{(l)}[j] = \bW{l}[j,\y]$.

\section*{Appendix C: Remarks}
\paragraph{Relation to \bf{FCM}} % \newcite{Mo-Yu:2014qv}}
The recently proposed Factor-based Compositional Model (\fcm)~\cite{Mo-Yu:2014qv} is a special case of \lrfcmtngram. 
% In \fcm~each word is represented each word in a structure with its word embedding vector and non-lexical feature vector,  then use the outer product between the two vectors to combine their information.
In particular, if we restrict ourselves to features with only one lexical part and set $\bW{e}=\bW{f}=\bW{\y}=\I$ to be identity matrices, we get the \fcm~model. Then using the scoring function in (\ref{eq:fcm_ngram}) gives: 
% which is given by:
\begin{align}
  \textstyle P(\y | \bx;\be, \cT) \propto \exp(\sum_i \cT_\y \odot (\mathbf{u_i} \otimes e_{\w_i})), \nonumber
\end{align}
where $\mathbf{u_i}$ is all non-lexical properties associated with $\w_i$.
\SideNoteRA{Not sure if I completely understand the math here; also the notation is not very clear. What is the type of $T$? Is it a matrix? Are we trying to relate it to $\cT$?}
\SideNoteMY{Is this version better?}
For each label $\y$, $\bx$ is scored with matrix $\cT_\y$.
All $\cT_\y$s form a tensor parameter $\cT=[\cT_1: \cdots :\cT_{\vert L\vert}]$. 
If we treat the pre-trained word embeddings as input, then \fcm{}
is equivalent to our model without low-rank approximations.
%The model parameters form a tensor $T=[T_1: \cdots :T_{\vert L\vert}]$. 
%which transforms the input matrix to labels.

Compared to our method, \fcm\ ignores dimensionality reduction for non-lexical properties and labels, making its usage of features and labels minimal. On the other hand, our model better suits the common setting in NLP, where we need to consider rich features, both lexical and non-lexical, and open-domain tasks with large label sets such as \newcite{hoffmann-zhang-weld:2010:ACL}. 
% We will further compare the two models in Remark2.

%We may view the scoring function in equation~(\ref{eq:fcmcp_ngram}) as a special case of scoring function in equation~(\ref{eq:fcm_ngram}) with a super-diagonal core tensor ($g_{i_1i_2\ldots i_K} = 1$ only if $i_1=i_2=\ldots=i_K$, otherwise $g_{i_1i_2\ldots i_K} = 0$) and with $r_1=\cdots=r_{n+2}=r$.
% and make transformation on each view has the same size of output $r$. 
%We call this model low-rank \fcm\ with multiple lexical parts (\lrfcmngram).

%For Remark2, setting $d=20$ for non-lexical feature embeddings gives the best performance. This view has highest dimensionality (if not fine-tuning word embeddings as in the Phrase Similarity task) so it actually dominates the number of parameters for lexical features with one word. We will report the best dimensionality for each view to make it more intuitive.
\paragraph{Representation size}
%\subsection{Effects on Dimension Reduction}
%\label{ssec:comparison}
Compared to  \fcm{}, \lrfcmt\ and \lrfcmcp\ result in a dramatic reduction in the number of model parameters (see Table \ref{tab:models} for details).
Consider the case of relation extraction in \S\ref{sec:exp}, which has 32 labels, 264 different non-lexical properties, and 200 dimensional word embeddings.  \fcm\ has  $1.7 \times 10^6$ parameters. In contrast, \lrfcm$_1${\sc -tucker} ($r_1$=32, $r_2$=20, $r_3$=200) and \lrfcm$_1${\sc -cp} ($r$=200 for all views) have 
$1.7 \times 10^5$ and $9.9 \times 10^4$ parameters, respectively. 
In the case of multi-word features, e.g. bigram features ($n=2$),
the number of parameters increase by two order of magnitude for
\lrfcm$_2${\sc -tucker} to $2.6 \times 10^7$ parameters, while only slightly for 
\lrfcm$_2${\sc -cp} to $1.4 \times 10^5$. 
Furthermore, 
the embeddings of non-lexical properties and labels can capture correlations among lexical features, further improving generalization. \SideNoteRA{Not sure what you mean.}
\SideNoteMD{The order of the numbers was reversed. Please check that my corrected text is correct.}
\SideNoteMY{I think the numbers are correct?}

\begin{table*}[tb]
  \small
  \centering
  %\begin{tabular}{|l|p{1.7cm}|p{2.9cm}|p{5.8cm}|}
  \begin{tabular}{|l|c|c|c|}
  \hline
    \multicolumn{1}{|c|}{} & {\bf Tensor Rank} & {\bf Number of Parameters} & {\bf Complexity during Prediction}\\
     \hline
    Full Tensor Model  &$d_1, d_2, d_3,\ldots, d_3$ & $d_1 \times d_2 \times d_3^n$ & $O(1)$ \\
    \fcm \cite{Mo-Yu:2014qv} &$d_1, d_2, d_{e},\ldots, d_{e}$ & $d_1 \times d_2 \times d_e^n$ & $d_1 \times d_2 \times d_e^n$ \\
    \hline
    \lrfcm$_n${\sc -tucker} (\S \ref{sec:lr_model_tucker}) & $r_1,r_2,r_3,\ldots,r_3$  & $r_1 \times r_2 \times r_3^n + d_1 r_1 + d_2r_2 + d_er_3$ &  $r_1 \times r_2 \times r_3^n$ 
    \\ 
    \lrfcm$_n${\sc -cp} (\S \ref{ssec:lr_ngram}) & $r$ & $r(d_1+d_2+d_e)$ & $(n+1) \times r$\\
%    \lrfcmcpsp (\S \ref{ssec:lr_structured}) & $r$ & $rd + s(m_2+m_3)$ & (n+1) * r \\ 
    \hline
  \end{tabular}
  \vspace{-.1in}
  \caption{\small{
    Comparison of different tensor models based on lexical features with $n$ lexical parts. $d_1$ and $d_2$ are the number of labels and features, respectively, $d_3$ is the size of word vocabulary, $d_e$ is the dimension of pre-trained word embeddings. For simplicity, we assume that the tensor rank for all lexical parts is equal to $r_3$ for \lrfcmt~and for \lrfcmcp~$r_1=r_2=r_3=\ldots=r_{n+2}=r$. 
% Here $n$ in \lrfcm$_n$ denotes the number of lexical parts.
%  As discussed in \S \ref{ssec:lr_ngram}, words on different views shares the same transformation so all lexical parts will be mapped to $r_1$-dimensional vectors. 
%  $s$ is the average number of non-zero elements of feature embeddings in \S \ref{ssec:lr_structured}. 
  % Here the time for looking up the embedding is ignored due to the efficiency of hash tables.
  % We can also get rid the time cost of mapping the pre-trained $d_e$-dimensional word embeddings to $r_3$-dimensional ones with pre-computing.  
We ignore the time for looking up the word embedding due to the efficiency of hash tables. We also ignore the cost of mapping pre-trained $d_e$-dimensional word embeddings to $r_3$-dimensional ones with pre-computing.  
  }
  }
  \vspace{-.1in}
  \label{tab:models}
%    \vspace{-1.5em}    
\end{table*}

\section*{Appendix C: Features for Relation Extraction}

To make fair comparison, we use the same non-lexical features in \cite{Mo-Yu:2014qv}.
\tabref{tab:fea_re} shows these features.
Note that those are only the non-lexical parts of the lexical features we hope to deal with.
Since in this task we only work on unigram lexical features, each lexical feature has its lexical part
which is any word in the training instance.
Therefore
the equivalent \emph{original lexical features} corresponding to these non-lexical feature templates are {\emph{the conjunctions among
a non-lexical feature generated by the templates in \tabref{tab:fea_re}, a word to which the non-lexical feature is associated, and the relation type}}.
\paragraph{Note:}
Here we show only the non-lexical feature template for tasks since the features in this task have unique number (1) of lexical parts. For n-gram features with mixed 
lengths (PP-attachment and preposition disambiguation), we will also show the original feature space
to better show that how we did factorization on features with different number of lexical parts.

The features in our relation extraction task are all unigram features, so in the table, each non-lexical property is defined on a word $w_i$. We denote the two target
entities as $M_1, M_2$, and their dependency path as $P$.
Here $h_1,h_2$ are the indices of the two head words of
$M_1,M_2$,
$\times$ refers to Cartesian product between two sets, $t_{h_1}$ and
$t_{h_2}$ are named entity types of the head
words of two entities, and $\phi$ stands for empty feature.
$\oplus$ refers to the conjunction of two elements.
%$\oplus$ refers to the combination of two elements.
%The second set plus the template in the first row of the first set are equivalent to the lexical features used in \cite{zeng-EtAl:2014:Coling}, while the other feature templates are first proposed in this paper.
The \feat{In-between} features indicate whether a word $w_i$ is in
between two target entities, and the \feat{On-path} features indicate
whether the word is on the dependency path, on which there is a set of words $P$, between the two entities. 

\begin{table}[htbp]
\centering
\scriptsize
\begin{tabular}{|l|c|}
\hline
\bf Set & \bf Template\\
\hline
\feat{HeadEmb} & $\{I[i=h_1], I[i=h_2]\}$ (head of $M_1/M_2$) \\
&  $\times \{\phi, t_{h_1},t_{h_2},t_{h_1}\oplus t_{h_2}\}$\\
\hline
\feat{Context} &  $I[i=h_1\pm 1]$ (left/right token of $w_{h_1}$) \\
&  $I[i=h_2\pm 1]$ (left/right token of $w_{h_2}$) \\
\hline
 \feat{In-between}  & $I[i > h_1] \& I[i < h_2]$ (in between ) \\
 & $\times \{\phi, t_{h_1},t_{h_2},t_{h_1}\oplus t_{h_2}\}$\\
 \hline
 \feat{On-path} & $I[w_i \in P]$ (on path)  \\
 & $\times \{\phi, t_{h_1},t_{h_2},t_{h_1}\oplus t_{h_2}\}$ \\
 \hline
\end{tabular}
\caption{Non-lexical feature templates for relation extraction.}
\label{tab:fea_re}
\vspace{-.8em}
\end{table}

\section*{Appendix D: Details for Experiments on PP-attachment}
\paragraph{Ranking-based Learning Objective:}
The PP-attachment task aims to select the correct head (verbs or nouns) from
a list (with varying sizes) of previous words in the sentence.
That is equivalent to give the current head highest rank in the list, therefore we formulate
the task as a ranking problem. Since there are less than 10 candidates, 
we adopt a list-wise training scheme. Given a 
preposition $p$ and its child $\w_c$, we minimize the loss of selecting
the correct head $\w_h$ from the candidate list $L$:
\begin{align}
 -\log \left( \frac{ \exp\left \{ s(\w_h,\w_p,\w_c) \right \} }{\sum_{\w_{h'}} \exp\left \{ s(\w_{h'},\w_p,\w_c) \right \} } \right). \nonumber
\end{align}
Therefore there is no view about labels in this task. Since for different candidate head $\w_h$,
the non-lexical parts for features associated to $\w_c$ may also change
(e.g. the distance feature in Table \ref{tab:fea_ppa_unigram}}),
the non-lexical parts for unigram features associated to $\w_c$ will not only depend on $\w_c$,
but also on the selection of $\w_h$.
To reflect this, we denote the set of non-lexical parts as $\mathbf{u}^{(1)}_{(\w_h,\w_p,\w_c)}(\v)$ for each word $\v$.
%, making the non-lexical feature set $\mathbf{u}=\mathbf{u}_{(w_h,p,w_c)}$. 
%Non-lexical parts for bigram features will have the form or $\mathbf{u}^{(2)}(\w_h,\w_c)$
%$\bh_{\x}^{(f)}$  
The scoring function for unigram features in equation
(\ref{eq:train-equivalent}) becomes:
\begin{align}
%&s(\y,\bx;\cT) = \sum_{\v=\{p,c\}} g \times_y \bh_{\y}^{(l)} \times_f \bh_{\mathbf{u}_{h,y}} \times_w \bh_{c}^{(1)}\nonumber .
&s(\y,\bx;\cT) = \sum_{\v \in \{\w_h,\w_c\}} \cT \times_f \mathbf{u}^{(1)}_{(\w_h,\w_p,\w_c)}(\v) \times_w \v\nonumber,
%&  = \exp\left \{ (g \times_y \bh_y)  \odot \left( \sum_i \bh_{\mathbf{f}_{w_i}} \otimes \bh_{e_{w_i}} \right) \right \}
\end{align}
and the function for bigram features is
\begin{align}
%&s(\y,\bx;\cT) = \sum_{\v=\{p,c\}} g \times_y \bh_{\y}^{(l)} \times_f \bh_{\mathbf{u}_{h,y}} \times_w \bh_{c}^{(1)}\nonumber .
&s(\y,\bx;\cT) = \cT \times_f \mathbf{u}^{(2)}(\w_h,\w_c) \times_{w_1} \w_h \times_{w_2} \w_c \nonumber.
%&  = \exp\left \{ (g \times_y \bh_y)  \odot \left( \sum_i \bh_{\mathbf{f}_{w_i}} \otimes \bh_{e_{w_i}} \right) \right \}
\end{align}

\paragraph{Feature Templates:}
Table \ref{tab:fea_ppa_original} shows the full set of original lexical features for this task.
Table \ref{tab:fea_ppa_unigram} \& \ref{tab:fea_ppa_bigram} listed the corresponding non-lexical
parts of the feature templates used for the \lrfcm$_1${\sc-tucker} and the \lrfcm$_2${\sc-cp} models. 
The non-lexical properties defined are similar for both models,
except that in the \lrfcm$_1${\sc-tucker} model, each feature contains only one word,
so we use an additional marker $c(w)$ to highlight the syntactic role $w$ plays, i.e.
whether $w$ is the child or a candidate head of the proposition word $w_p$.
While the bigram \lrfcm$_2${\sc-cp} model can already distinguish the child and head since
they belong to different views of the tensor,
so the $c(w)$ function is not in need.

%For the unigram model, the equivalent \emph{original lexical features} are {\emph{the conjunction 
%between a non-lexical feature, a word to which the non-lexical feature is associated}}.
%For the bigram model, the equivalent \emph{original lexical features} are {\emph{the conjunction 
%among a non-lexical feature, and the pair of words to which the non-lexical feature is associated}}.

\paragraph{Baseline Methods:}
Besides the traditional SVMs and the HPCD methods proposed in \newcite{belinkov2014exploring}, we also compared with
several state-of-the-art parsers and re-rankers on this task.
The parsers include: Malt \cite{nivre2006maltparser}, MST \cite{mcdonald2005online}, Turbo \cite{martins2013turning} and RBG \cite{lei-EtAl:2014:P14-1}.
The re-rankers include a recursive neural network (RNN) based re-ranker \cite{socher2013parsing} and 
the one from \newcite{mcclosky2006effective}.
The full results can be found in Table \ref{tab:fullres_ppa}.

\begin{table}[htbp]
\small
\centering
	\begin{tabular}{|c|c|}
	\hline
	\bf Set &{\bf Template}  \\
	\hline
	Bag of Words & $w$ ($w$ is $w_m$ or $w_h$), $w_m \& w_h$\\
	Distance & Dis$(w_h, w_m)$ $\&$ $\{w_m, w_h, w_m \& w_h\}$\\
	Prep & $w_p$ $\&$ $\{w_m, w_h, w_m \& w_h\}$\\
	POS & $t(w_h)$ $\&$ $\{w_m, w_h, w_m \& w_h\}$\\
	NextPOS & $t(w_{h+1})$ $\&$ $\{w_m, w_h, w_m \& w_h\}$ \\
	{VerbNet} & $P=\{p(w_h)\}$ $\&$ $\{w_m, w_h, w_m \& w_h\}$\\
	& $I[w_p \in P]$ $\&$ $\{w_m, w_h, w_m \& w_h\}$\\
	WordNet & $R_h=\{r(w_h) \}$ $\&$ $\{w_m, w_h, w_m \& w_h\}$\\
	& $R_m=\{r(w_m) \}$ $\&$ $\{w_m, w_h, w_m \& w_h\}$\\
	\hline
	\end{tabular}
\caption{\small Original feature templates for PP-attachment task: 
Each feature is defined on tuple ($w_m$, $w_p$, $w_h$), where $w_p$ is the preposition word,
$w_m$ is the child of the preposition, and $w_h$ is a candidate head of the preposition.
%$m$ and $h$ are the absolute positions of the two words in a sentence. 
$t(w)$: POS tag of word $w$; $p(w)$: the preposition defined in the frames of verb $w$ from VerbNet; $r(w)$: the root hypernym of word $w$ defined in WordNet. Dis$(w_h, w_m)$ indicates the number of candidate heads between $w_h$ and $w_m$. 
%$\times$ refers to Cartesian product between two sets
}
\label{tab:fea_ppa_original}
\end{table}

\begin{table}[htbp]
\small
\centering
	\begin{tabular}{|c|c|}
	\hline
	\bf Set &{\bf Template}  \\
	\hline
	Bias & b\\	
	Distance & Dis$(w_h, w_m)$ $\&$ $c(w)$ \\
	Prep & $w_p$ $\&$ $c(w)$ \\
	POS & $t(w_h)$ $\&$ $c(w)$ \\
	NextPOS & $t(w_{h+1})$ $\&$ $c(w)$  \\
	{VerbNet} & $P=\{p(w_h)\}$ $\&$ $c(w)$\\
	& $w_p \in P$ $\&$ $c(w)$\\
	WordNet & $R_h=\{r(w_h) \}$ $\&$ $c(w)$ \\
	& $R_m=\{r(w_m) \}$ $\&$ $c(w)$ \\
	\hline
	\end{tabular}
\caption{\small Non-lexical feature templates for PP-attachment task (unigram model): 
The definition of the symbols are same to those in Table \ref{tab:fea_ppa_original}.
Each non-lexical feature is associated to a word $w$ in pair ($w_m$,$w_h$).
$c(w)$ is a map from $w$ to the set of syntactic roles $\{C, H\}$, where $c(w)=C$ indicates $w=w_m$,
and $c(w)=H$ indicates $w=w_h$. This feature is used to distinguish different functions 
of a non-lexical feature when it is associated to the child or the head.}
\label{tab:fea_ppa_unigram}
\end{table}

\begin{table}[htbp]%[!h]
\small
\centering
	\begin{tabular}{|c|c|}
	\hline
	\bf Set &{\bf Template}  \\
	\hline
	Bias & b\\
	Distance & Dis$(w_h, w_m)$  \\
	Prep & $w_p$ \\
	POS & $t(w_h)$ \\
	NextPOS & $t(w_{h+1})$   \\
	{VerbNet} & $P=\{p(w_h)\}$ \\
	& $w_p \in P$ \\
	WordNet & $R_h=\{r(w_h) \}$\\
	& $R_m=\{r(w_m) \}$  \\
	\hline
	\end{tabular}
%\caption{Feature templates for word $w_i$ in phrase $p$. $t(w)$: POS tag; $c(w)$: word cluster; $h$: position of head word of the phrase $p$; Dis$(i-j)$: distance between $w_i$ and $w_j$.}
\caption{\small Non-lexical feature templates for PP-attachment task (bigram model): 
The definition of the symbols are same to those in Table \ref{tab:fea_ppa_original}.
Each non-lexical feature is associated to a pair ($w_m$,$w_h$).
Here each feature is associated to word pair so we
do not need the $c(w)$ function in Table \ref{tab:fea_ppa_unigram} to indicate the syntactic role of a single target word.}
\label{tab:fea_ppa_bigram}
\end{table}

\begin{table*}[htbp]
\centering
\small
\begin{tabular}{|l|c|c|c|}
\hline
\bf System & \bf Resources Used & \bf Acc\\
\hline
Closest  & distance & 81.7 \\
\hline
\multirow{1}{*}{SVM}  & distance, word, embedding, clusters, POS, WordNet, VerbNet &\multirow{1}{*}{86.0} \\
%\multirow{1}{*}{SVM} & smoothed full features & distance, clusters, POS, WordNet, VerbNet &\multirow{1}{*}{} \\
\hline
Malt & \multirow{4}{*}{dependency parser} & 79.7 \\
MST & & 86.8\\
Turbo  &  & 88.3\\
RBG & & 88.4\\
\hline
RNN & re-ranker, embedding &85.1 \\
Charniak-RS  & re-ranker & 88.6\\
\hline
%{HPCD (basic)} && 85.4\\
HPCD  &distance, embedding, POS, WordNet, VerbNet&{88.7}\\
\hline
RBG + HPCD & dependency parser, compositional model& \multirow{1}{*}{90.1}\\
\hline
\multirow{1}{*}{\lrfcm$_1${\sc-tucker}}   & distance,embedding, POS, WordNet,VerbNet  & 89.3 \\ %87.85 \\
%& + POS,next POS,VerbNet  & 90.1 \\ %90.06\\
%\hline
\multirow{1}{*}{\lrfcm$_2${\sc-cp}} & distance, embedding, POS, WordNet, VerbNet  &  89.2\\
%& + POS,WordNet,VerbNet & 90.1\\ %90.12\\
\hline
{\lrfcm$_1${\sc-tucker}} \& {\lrfcm$_2${\sc-cp}} & distance, embedding, POS, WordNet, VerbNet & \multirow{1}{*}{\bf 90.3}\\ % \multirow{2}{*}{\bf 90.52}\\
\hdashline
{\lrfcmcluster}  & distance, embedding, clusters, POS, WordNet, VerbNet & \multirow{1}{*}{89.9}\\ 
\hline
\end{tabular}
\caption{\small PP-attachment test accuracy.} 
\label{tab:fullres_ppa}
%\vspace{-.5cm}
\end{table*}

\begin{table*}[htbp]
\centering
\small
\begin{tabular}{|l|c|c|}
\hline
 \bf Features & \bf HPCD & \bf {\lrfcm$_1${\sc-tucker} \& \lrfcm$_2${\sc-cp}}\\
\hline
w2m embedding & 85.4 & 85.9\\%87.9\\
+ POS & 86.4 & 86.1\\%89.1 \\ %89.08\\
+ NextPOS & 87.5 & 87.4\\%89.6\\
+ WordNet+VerbNet & 87.7 & 87.9\\% 89.8\\
\hline
all features + fine-tuning & 88.1 & 88.7\\% 90.01 \\
\hline
all features + fine-tuning + syn embedding& \multirow{1}{*}{88.7} &\multirow{1}{*} {\bf 90.1}\\% \multirow{2}{*}{90.06}\\
all features + syn embedding& \multirow{1}{*}{ - } &\multirow{1}{*} {\bf 90.4}\\
%& + POS,VerbNet &89.49\\
%& + WordNet & 88.67\\
%& + POS,next POS,VerbNet & 90.11\\
%& + all & \\
\hline
\end{tabular}
\caption{\small Ablation comparisons for HPCD and \lrfcm{}.} 
\label{tab:pp_res_abla2}
\end{table*}

\begin{table}[htbp]%[!h]
\small
\centering
	\begin{tabular}{|c|c|c|}
	\hline
	\bf Set &{\bf Template} \\
	\hline
	Bag of Words & $w$, $p$ $\&$ $w$ ($w$ is $w_m$ or $w_h$)\\
	Words \& positions & $w_m$, $w_h$, $w_m$ $\&$ $w_h$ \\
	Preposition& $p$, $p$ $\&$ $w_{m}$, $p$ $\&$ $w_h$, $p$ $\&$ $w_m$ $\&$ $w_h$ \\
	\hline
	\end{tabular}
\caption{\small Original feature templates for each preposition word $p$ and its modifier noun $w_m$ and head noun $w_h$ in the sentence. The bag-of-words features ignore the positions of each word.
Since the sentences are different from each other on only $p$, $w_m$ and $w_h$, for all the lexical features we ignore the words on the other positions.}
\label{tab:fea_preposition}
\end{table}

\paragraph{Full Results and Ablation Tests:}
The full results on this task are included in \tabref{tab:fullres_ppa}.
The table lists all the results from \newcite{belinkov2014exploring} for comparison.
It also lists the performances of \lrfcm{}s using only unigram features (\lrfcm$_1${\sc-tucker})
and bigram features (\lrfcm$_2${\sc-cp}).
These two models with reduced feature sets can still outperform all the other single systems,
including HPCD. We also observe a large improvement when using both type of features (from 89.3 to 90.3). Such a result confirmed the importance of using higher-order $n$-gram lexical features, and the advantage of our proposed methods in \S\ref{sec:lr_model_ngram}.

We include ablation tests (\tabref{tab:pp_res_abla2}) on the test set in order to compare with the HPCD 
results from \newcite{belinkov2014exploring}. 
Similar to their findings, the POS tag of the word next to candidate head
contributes most to performance. 
\lrfcm\ and HPCD achieve similar scores when the word2vec embeddings (w2m) are used.
Under this setting, \lrfcm\ obtains higher improvements when fine-tuning is enabled.
This is because that \lrfcm\ with w2m embeddings under-fit the data since the embeddings are not
discriminative enough.%while the HPCD is a non-linear model.
In this case fine-tuning can make the embeddings more task-specific so it improves the result.
When the syntactic embeddings (syn) are used, the \lrfcm\ performs significantly better, due to the better usage of linguistic features. Note that in this case the model is sufficient powerful so enabling
fine-tuning only increases the risk of over-fitting (90.1 v.s. 90.4).
%We find that for every feature setting, \lrfcm\ can consistently improve over HPCD.

%\section*{Appendix E: Statistics of the Tasks}
%
%Table \ref{tab:exp_stats} shows the statistics of each task.
%
%\begin{table*}[htbp]
%\centering
%\small
%\begin{tabular}{|l|c|c|c|c|}
%\hline
%\multirow{2}{*}{\bf Task} & \multirow{2}{*}{\bf Benchmark} & \multirow{2}{*}{\bf Dataset} & \multicolumn{2}{|c|}{\bf Numbers on Each View} \\
%	\cline{4-5}
%       & &  & \bf \#Labels ($m_3$) & \bf \#Unlexical Features ($m_2$)\\
%       \hline
%       Relation Extraction & - & ACE 2005 & 32 & 264 \\
%%       \hline
%       Phrase Similarity & - & PPDB & 10,000 & 2,354 \\
%%       \hline
%      PP-attachment & \cite{belinkov2014exploring} & WSJ & - & 1,213 / 607 \\
%       %joint-\lrfcm\ (ST) &  & \textbf{} &   \\
%        \hline
%\end{tabular}
%\caption{\small Statistics of each task. For PP-attachment task, we have models for unigram features and bigram features. Therefore we list the numbers of features for both model. The bigram model has half number of features as the unigram model has (excluding the bias feature), because there is no need to indicate whether the role ($c(w)$) of a word is the child (C) or head (H).} 
%\label{tab:exp_stats}
%%\vspace{-.4cm}
%\end{table*}

\section*{Appendix E: Features for the Preposition Disambiguation Task}
We use the lexical features in \tabref{tab:fea_preposition} for this task.
The templates contains bigram lexical features, so similar to the PP-attachment task,
we can use the combination of a \lrfcm$_1$ and a \lrfcm$_2$,
or use a single \lrfcmcluster, to represent the whole feature sets.

\removed{
\section*{Appendix F: Experiments on Phrase Similarity}
\paragraph{Experimental Setting:}
We evaluate on the bigram-to-unigram similarity task in \cite{TACL586}.
The task is to match a bigram noun phrase with a noun word from the Paraphrase Database (PPDB)\footnote{\url{http://www.cis.upenn.edu/~ccb/ppdb/}} \cite{ganitkevitch2013ppdb}.
%We removed all the pairs in which the phrase is composed by an article and a noun.
%PPDB is organized into 6 parts, ranging from S (small) to XXXL. Division into these sets is based on an automatically
%derived accuracy metric.
%Phrases were extracted from the XXL set, where the most accurate 1,000 pairs are used for evaluation and divided
%into a dev set (500 pairs) and test set (500 pairs); the remaining pairs were used for training. 
We use the same training/dev/test split in \cite{TACL586}, evaluate by ranking top 10k words for a query phrase and report mean reciprocal rank (MRR).

Since the output labels of this task are 10k possible nouns,
the number of labels $d_1$ requires the use of label embeddings.
\SideNoteMY{No such experiments currently}
Since 
phrase semantics depend on the combination of component words,
we expect the conjunction of multiple component word embeddings to help.
Additionally, evaluating on bi-gram phrases allows us to test our model that uses multiple lexical parts (\lrfcmngram).

We compare to two baselines in \cite{TACL586}: 
point-wise addition (SUM) \cite{mitchell2010composition}
and a recursive neural network model (RNN) \cite{socher2013parsing}   
with 50 and 200 dimensional embeddings.

For hyper-parameters tuning of \lrfcmt, we use same setting as in \emph{relation extraction},
but choose $r_1$ from $\{50,100,200\}$.
For \lrfcmcp, we select $r=\{50,100,200\}$. We also try fine-tuning of the original
$d$-dimensional word embeddings, which performs better on dev than
using fixed embeddings.

\paragraph{Feature Template:}
Our non-lexical feature templates are shown in \tabref{tab:fea_ppdb}. 
The equivalent \emph{original lexical features} they correspond to 
become {\emph{the conjunction among
a non-lexical feature, a word to which the non-lexical feature is associated, }and \emph{the target word}}.
Phrase boundaries, tags and heads are identified
using existing parsers or from Annotated Gigaword \cite{napoles2012annotated}.
Following the evaluation task we experimented with bigram NPs so this table only focuses on non-lexical features for the noun phrase with one modifier word $w_m$ and one head word $w_h$. We leave explorations of features for complex structures to future work. 

\begin{table}[htbp]%[!h]
\small
\centering
	\begin{tabular}{|c|c|c|}
	\hline
	\bf Set &{\bf Template} \\
	\hline
	Bias & b\\
	POS tags& $t(w_{m})$, $t(w_h)$ \\
	&   $t(w_{m}) \& t(w_{h})$  \\
	Word clusters & $b(w_{m})$, $b(w_h)$ \\
	&   $b(w_m) \&  b(w_h)$ \\
	Head word & $I[i=h]$   \\
	&   $t(w_{k}) \& I[i=h]$ $k\in\{i-1,i,i+1\}$ \\
	&   $b(w_{k})\& I[i=h]$ $k\in\{i-1,i,i+1\}$\\
	\hline
	\end{tabular}
%\caption{Feature templates for word $w_i$ in phrase $p$. $t(w)$: POS tag; $c(w)$: word cluster; $h$: position of head word of the phrase $p$; Dis$(i-j)$: distance between $w_i$ and $w_j$.}
\caption{\small Non-lexical feature templates for each word $w$ in phrase $p$. We denote the modifier as $w_m$ and the head as $w_h$. $t(w)$: POS tag; $b(w)$: word cluster; $h$: position of head word of the phrase $p$.
Bias means a constant feature for each word in any situation.
If we only have the bias feature then the model will reduce to point-wise summation.}
\label{tab:fea_ppdb}
\end{table}

\paragraph{Results:}
Table \ref{tab:res_ppdb} confirms the observation of \newcite{blacoe-lapata:2012:EMNLP-CoNLL}
that compositional models (RNNs) do worse than SUM.
On the other hand, both of our \lrfcm\ models perform better than SUM.
In this task, the label set is exactly the word vocabulary, each lexical feature we used
is actually a bigram feature (as a result we denote all our methods as \lrfcm$_2$). 
In this case, \lrfcmcp\ does a better job of handling features with
multiple lexical parts. This is the only task that fine-tuning word embeddings $\be$ helps,
indicating that the pre-trained word embeddings may contain sufficient syntactic information
of words but not doing so well on their semantics. It is interesting that the best \lrfcm$_2${\sc -cp} 
($r$=200 and $\bW{3}=\mathbf{I}$)
on dev set is equivalent to the proposed FCT model in \cite{TACL586}, confirming the advantage of
this choice of models on the phrase similarity task.

\begin{table}[htbp]
\centering
\small
\begin{tabular}{|l|c|c|}
\hline
\multirow{1}{*}{ \bf Method} &  \multirow{1}{*}{\bf MRR@10k}\\
\hline
%SUM & N &31.40\\
%Recursive NN (d=50) & N & 30.51\\
%Recursive NN (d=200)  & N & 34.25\\
%\lrfcmcp (unigram) & N & 33.99\\
%\lrfcmt (unigram)  & N & 33.84\\
%\lrfcm (bigram)  & \\
%\lrfcm (combine)  & \\
SUM &41.19\\
Recursive NN (d=50) &  39.25\\
Recursive NN (d=200)  & 40.50\\
\lrfcm$_2${\sc -cp} (bigram)  & \bf 44.31\\
\lrfcm$_2${\sc -tucker} (bigram)  & 42.22\\
%\lrfcm (bigram)  & \\
%\lrfcm (combine)  & \\
\hline
\end{tabular}
\vspace{-.1cm}
\caption{\small Phrase similarity test MRR.} 
\label{tab:res_ppdb}
\vspace{-.2cm}
\end{table}
}
